# Supplementary material for: From Recognition to Cognition: Visual Commonsense Reasoning
Source: arXiv:1811.10830 source file (2019-03-26)
Supplement: Supplementary file 1 [file supp.tex]

\documentclass[10pt,twocolumn,letterpaper]{article}

\usepackage{cvpr}
\usepackage{times}
\usepackage{epsfig}
\usepackage{graphicx}
\usepackage{amsmath}
\usepackage{amssymb}
\usepackage{caption}
\usepackage{bm}

\usepackage{booktabs}
\usepackage{algorithm}
\usepackage{algorithmic}
\usepackage{graphicx}
\usepackage{enumitem}
\usepackage{multirow}
\usepackage{caption}
\usepackage[normalem]{ulem}
\usepackage{xcolor,colortbl, makecell}
\usepackage{afterpage}
\usepackage{placeins}

\newcommand{\com}[1]{}
  % defining a new term
   % vector var
    % matrix var

\usepackage{amsmath}  % required if you use \overset

% Include other packages here, before hyperref.

% If you comment hyperref and then uncomment it, you should delete
% egpaper.aux before re-running latex.  (Or just hit 'q' on the first latex
% run, let it finish, and you should be clear).
\usepackage[pagebackref=true,breaklinks=true,letterpaper=true,colorlinks,bookmarks=false]{hyperref}

% \cvprfinalcopy % *** Uncomment this line for the final submission

 % *** Enter the CVPR Paper ID here

% Pages are numbered in submission mode, and unnumbered in camera-ready
\ifcvprfinal\pagestyle{empty}\fi
\begin{document}

%%%%%%%%% TITLE
% \title{zLooking Beyond the Frame: Commonsense Inference about the Visual World}
% \title{Answering and Justifying Visual Commonsense Inferences}
% \title{Commonsense Visual Question Answering and Justification}
% \title{Answering and Justifying commonsense Commonsense Visual Question Answering and Justification}
%\title{Visually Grounded Commonsense Inference}
% \title{Visual Commonsense Reasoning}
\title{From Recognition to Cognition: Visual Commonsense Reasoning (supplemental material)}

% Rowan, Yonatan, Ali, Yejin
\author{Rowan Zellers$^\spadesuit$ \: \: 
  Yonatan Bisk$^\spadesuit$ \: \:
  Ali Farhadi$^{\spadesuit\heartsuit}$ \: \:
  Yejin Choi$^{\spadesuit\heartsuit}$\\
  $^\spadesuit$Paul G. Allen School of Computer Science \& Engineering, University of Washington \\
  $^\heartsuit$Allen Institute for Artificial Intelligence
  }

% \author{First Author\\
% Institution1\\
% Institution1 address\\
% {\tt\small firstauthor@i1.org}
% % For a paper whose authors are all at the same institution,
% % omit the following lines up until the closing ``}''.
% % Additional authors and addresses can be added with ``\and'',
% % just like the second author.
% % To save space, use either the email address or home page, not both
% \and
% Second Author\\
% Institution2\\
% First line of institution2 address\\
% {\tt\small secondauthor@i2.org}
% }

\maketitle
\thispagestyle{plain}
\pagestyle{plain}

%%%%%%%%% ABSTRACT
%%%%%%%%% BODY TEXT

\vspace{-10pt}

%%%%%%%%% TITLE
% \title{zLooking Beyond the Frame: Commonsense Inference about the Visual World}
% \title{Answering and Justifying Visual Commonsense Inferences}
% \title{Commonsense Visual Question Answering and Justification}
% \title{Answering and Justifying commonsense Commonsense Visual Question Answering and Justification}
%\title{Visually Grounded Commonsense Inference}
% \title{Visual Commonsense Reasoning}
\title{From Recognition to Cognition: Visual Commonsense Reasoning (supplemental material)}

% Rowan, Yonatan, Ali, Yejin
\author{Rowan Zellers$^\spadesuit$ \: \: 
  Yonatan Bisk$^\spadesuit$ \: \:
  Ali Farhadi$^{\spadesuit\heartsuit}$ \: \:
  Yejin Choi$^{\spadesuit\heartsuit}$\\
  $^\spadesuit$Paul G. Allen School of Computer Science \& Engineering, University of Washington \\
  $^\heartsuit$Allen Institute for Artificial Intelligence
  }

% \author{First Author\\
% Institution1\\
% Institution1 address\\
% {\tt\small firstauthor@i1.org}
% % For a paper whose authors are all at the same institution,
% % omit the following lines up until the closing ``}''.
% % Additional authors and addresses can be added with ``\and'',
% % just like the second author.
% % To save space, use either the email address or home page, not both
% \and
% Second Author\\
% Institution2\\
% First line of institution2 address\\
% {\tt\small secondauthor@i2.org}
% }

\maketitle
\thispagestyle{plain}
\pagestyle{plain}

%%%%%%%%% ABSTRACT
%%%%%%%%% BODY TEXT

\vspace{-10pt}

% \section{Conclusion}
% \input{sections/08_conclusion.tex}

% \section{Stuff to go in the appendix}
\clearpage
{\small
\bibliographystyle{ieee}
\bibliography{cvpr2019}
}

% \section{Conclusion}
% \input{sections/08_conclusion.tex}

% \section{Stuff to go in the appendix}
\clearpage
{\small
\bibliographystyle{ieee}
\bibliography{cvpr2019}
}
\end{document}
